# Supplementary material for: SpeechCap: Leveraging Playful Impact Captions to Facilitate Interpersonal Communication in Social Virtual Reality
Source: arXiv:2502.10736 source file (2025-04-09)
Supplement: Supplementary file 1 [file appendix.tex]

% \section{Content Analysis on Videos with Impact Captions}
% ABCDEFG.

% \section{Workshop Output}
% ABCDEFG.

\section{Word Lists for Visual appearances}
\label{sec_appendix_words}

We use the following specified word lists to determine the visual appearances of impact captions in \system{}. 

\begin{table*}[hbt]
  \caption{The Word Lists used in \system{} for the Visual Design of Impact Captions}
  \Description{.}
  \label{tab:word_lists}
  \begin{tabular}{p{1.5cm}p{2cm}p{9cm}}
    \toprule
        Dimension & Semantic & Words  \\
    \midrule
        Typeface & formality & Grave, Critical, Severe, Intense, Urgent, Significant, Serious, Profound, Consequently, Nevertheless \\

        Emoji & smiling face & Happy, Nice, Cheerful, Joyful, Lovely, Grateful, Warm, Friendly, Sweet, Gentle, Pleasant, Fantastic, Smiling, Wonderful, Amazing, Positive, Hopeful, Heartwarming \\

        Emoji & sad face & Sad, Sadly, Sorrowful, Gloomy, Heartbroken, Miserable, Awful, Hopeless, Depressed, Lonely, Agonized, Distressed, Painful, Troubled, Crushed, Crying \\

        Emoji & embarrassed face & Embarrassed, Ashamed, Flustered, Uncomfortable, Nervous, Overwhelmed, Stumbling, Guilty, Shy, Flushed, Anxious \\

        Ornament & object & Apple, Building, Bicycle, Bread, Bird, Cake, Car, Cat, Clock, Dog, Food, Sun, Rain, Book, Phone, Computer, Building, Tree, Flower \\

        Speech Bubble & greetings & Hi, Hey, Hello, Howdy, Greetings, Heya, Hiya, Hola, Aloha. \\

        Speech Bubble & interjections & Shocked, Surprised, Thrilled, Wow, Bruh.  \\

        Motion & shivering & Shocking, Shocked, Shock, Surprising, Surprised, Surprise, Astonished, Stunned, Overwhelmed, Thrilled \\
    \bottomrule
\end{tabular}
\end{table*}
